# Supplementary material for: Distill Knowledge from NRSfM for Weakly Supervised 3D Pose Learning
Source: arXiv:1908.06377 source file (2019-08-18)
Supplement: Supplementary file 1 [file supp.tex]

\subsection{camera estimator $q_M(\W)$}
\cy{dump to appendix}
\label{sec:cam_est}
\begin{equation}
\begin{aligned}
\mathbf{S} = \D_1^\sharp (\bvarphi_1 \otimes \I_3), &~~~~ \|\bvarphi_1\|_1\leq\lambda_1, \bvarphi_1 \geq 0,\\
\bvarphi_1 \otimes \I_3= (\D_2 \otimes \I_3 ) (\bvarphi_2 \otimes \I_3), &~~~~ \|\bvarphi_2\|_1\leq\lambda_2, \bvarphi_2 \geq 0,\\
\vdots~~~~~~~~, &~~~~ \vdots\\
\bvarphi_{n-1} \otimes \I_3= (\D_n \otimes \I_3 ) (\bvarphi_n \otimes \I_3), &~~~~ \|\bvarphi_n\|_1\leq\lambda_n, \bvarphi_n \geq 0,\\
\end{aligned}
\end{equation}

multiply both sides by the camera matrix $\M$

\begin{equation}
    \begin{aligned}
    \W = \D_1^\sharp \bPsi_1,&~~~~\|\bPsi_1\|_1\leq\lambda'_1\\
    \bPsi_1 = (\D_2\otimes\I_3)\bPsi_2,&~~~~\|\bPsi_2\|_1\leq\lambda'_2\\
    \vdots~~~~~,&\\
    \bPsi_{n-1}=(\D_n\otimes\I_3)\bPsi_n,&~~~~\|\bPsi_n\|_1\leq\lambda'_n
    \end{aligned}
\end{equation}

\begin{equation}
\begin{aligned}
    \bPsi_1 = &\text{soft}((\D_1^\sharp)^T\W,~ \mathbf{b}_1\otimes\mathbf{1}_{3\times2})\\
    \bPsi_2 = & \text{soft}((\D_2\otimes\I_3)^T\bPsi_1,~\mathbf{b}_2 \otimes \mathbf{1}_{3\times2})\\
    \vdots & \\
     \bPsi_n = & \text{soft}((\D_n\otimes\I_3)^T\bPsi_{n-1},~\mathbf{b}_n \otimes \mathbf{1}_{3\times2})\\  
\end{aligned}
\end{equation}

\begin{equation}
    \min_{\M, \bvarphi_n} \|\bPsi_n - \bvarphi_n \otimes\M\|_2^2
\end{equation}

\begin{equation}
    \bPsi_n = [\mathbf{\Pi}^T_1, \dots, \mathbf{\Pi}^T_K]^T, ~~~~\bvarphi_n = [c_1, \dots, c_K]^T
\end{equation}

with $\bvarphi_n$ fixed:
\begin{equation}
    \tilde{\M} \propto \sum_{k=1}^K c_k \Pi_k
\end{equation}

with $\M$ fixed:
\begin{equation}
    \tilde{c_k} = \frac{1}{2}\text{grandsum}(\Pi_k \odot \M)
\end{equation}

\subsection{code estimator $q_\varphi(\W, \M)$}
\label{sec:code_est}
\cy{dump to appendix}

\begin{equation}
 \R = [\mathbf{m}_1, \mathbf{m}_2, \mathbf{m}_1 \times \mathbf{m}_2],   
\end{equation}

\begin{equation}
    \B = \begin{bmatrix}
    [\mathbf{d}_x^1, \mathbf{d}_y^1, \mathbf{d}_z^1]\R & \dots & [\mathbf{d}_x^P, \mathbf{d}_y^P, \mathbf{d}_z^P]\R
    \end{bmatrix}^T
\end{equation}

encoder:
\begin{equation}
    \begin{aligned}
    \bvarphi_1 & = \text{ReLU}(\B_{xy}^T\bw - \mathbf{b}_1),\\
    \bvarphi_2 & = \text{ReLU}(\D_2^T\bvarphi_1 - \mathbf{b}_2),\\
    & \vdots\\
    \bvarphi_n & = \text{ReLU}(\D_n^T\bvarphi_{n-1} - \mathbf{b}_n)\\
    \end{aligned}
\end{equation}
decoder:
\begin{equation}
    \begin{aligned}
    \bvarphi_{n-1} = & \text{ReLU}(\D_n\bvarphi_n-\mathbf{b}_n),\\
    & \vdots\\
    \bvarphi_1 = & \text{ReLU}(\D_2\bvarphi_2-\mathbf{b}_2),\\
    \end{aligned}
\end{equation}
